# Supplementary material for: Neural CRNs: A Natural Implementation of Learning in Chemical Reaction Networks
Source: arXiv:2409.00034 ancillary file (2025-09-08)
Supplement: Supplementary file 1 [file Neural_CRNs_ACS_Supplementary_V3.pdf]

# Neural CRNs: A Natural Implementation of Learning in Chemical Reaction Networks

Rajiv Teja Nagipogu<sup>1</sup>, John H. Reif<sup>1\*</sup>

<sup>1</sup>*Department of Computer Science, Duke University, 2127 Campus Drive, Durham, NC 27708*

E-mail: [rajivteja.nagipogu@duke.edu](mailto:rajivteja.nagipogu@duke.edu)

## S1 Supervised Learning in Feedforward Neural Networks

*Feedforward Neural Networks* (FFNNs; neural networks for short) are layered graph-like structures with directed weighted connections between nodes of neighboring layers. The weights of these connections serve as the *network parameters* and facilitate learning through gradient-based optimization methods.<sup>1,2</sup> These methods “train” the network by adjusting the parameters towards optimizing an objective function, such as minimizing a risk or maximizing a reward.

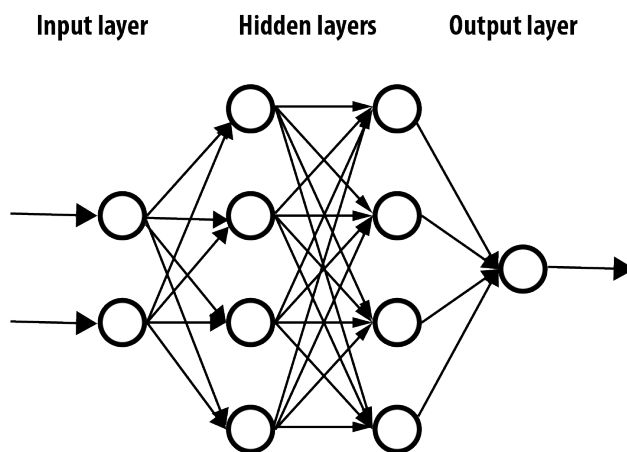

**Figure S1:** Schematic of a feedforward neural network that takes in two-dimensional input, consists of two hidden layers and outputs a scalar.

*Supervised learning* is one such learning approach, in which the network is optimized over a “labeled” dataset of input/output pairs. In this approach, the network is trained iteratively to learn a transformation function from the input space to the output space, such that the final transformation function can accurately predict the output corresponding to a previously unseen input.

Each iteration of supervised learning (corresponding to the input/output pair  $(\mathbf{x}, y)$ ) consists of two main phases: (i) the feedforward phase and (ii) the feedback phase. Briefly, the *feedforward* phase involves computing the network output  $\hat{y}$  given  $\mathbf{x}$  by transforming it sequentially through the layers of the network according to the current parameter set. The effective computation is represented using  $F_{\theta}^{\text{current}}$  as shown in eq. (1). The *feedback phase* involves computing the parameter gradients with respect to a loss function  $\frac{\partial \mathcal{L}}{\partial \theta}$ , where loss  $\mathcal{L}$  is defined as the error between  $\hat{y}$  and  $y$  (2). For this purpose, neural networks employ the *backpropagation* algorithm,<sup>1</sup> an efficient implementation of the chain rule for partial differentiation,<sup>3</sup> Finally, the current parameters are updated according to these gradients using the gradient descent formulation shown in eq. (3).

$$\hat{y} = F_{\theta}^{\text{current}}(\mathbf{x}) \quad (1)$$

$$\mathcal{L} = \text{error}(\hat{y}, y) \quad (2)$$

$$\theta^{\text{updated}} = \theta^{\text{current}} - \eta \frac{\partial \mathcal{L}}{\partial \theta}. \quad (3)$$

Here,  $\eta$  represents the learning rate that indicates how fast the network learns. This two-phase process is repeated over the entire dataset multiple times until the loss converges, after which the network is declared to be *trained* for the supervised learning task represented by the dataset. A more detailed mathematical description of the supervised learning procedure in neural networks is provided in SI Text S1.

## S2 Neural Ordinary Differential Equations

*Neural ordinary differential equations* (Neural ODEs)<sup>4</sup> are a continuous dynamical system-based implementation of learning and thus represent a conceptually different approach to neural computations in FFNNs. While FFNNs are discrete systems that utilize matrix transformations at discrete layers to perform the neural computations, Neural ODEs model them using the ODE evolution of their continuous state variables. These computations are then evaluated by solving the initial value problems (IVPs) of these ODE evolutions.<sup>5</sup>

Figure S2 depicts the supervised learning architecture in the Neural ODEs framework. Here, we consider a supervised learning task with input  $\mathbf{x} \in \mathbb{R}^n$  and the corresponding output  $\mathbf{y} \in \mathbb{R}^m$ . Recall that the computations in Neural ODEs are modeled as ODE evolutions, which means that they are dimension-preserving. Here, we assume that the dimensionality of the Neural ODE is  $d$ , i.e., its hidden state is a  $d$ -dimensional vector  $\mathbf{z} \in \mathbb{R}^d$ . Therefore, in order to align the inputs and outputs of the supervised learning task with Neural ODE dimensionality, two auxiliary linear projection layers  $W_{\text{in}}^{n \times d}$  and  $W_{\text{out}}^{d \times m}$  are included alongside the Neural ODE. Briefly,  $W_{\text{in}}$  effects a transformation from the input space to Neural ODE space, while  $W_{\text{out}}$  effects a transformation from Neural ODE space to the output space. Below, we describe the computations involved in the supervised learning procedure of the Neural ODEs framework. A summary of this procedure is provided in Table S1 for reference. We refer the reader to the original work<sup>4</sup> for a more detailed description.

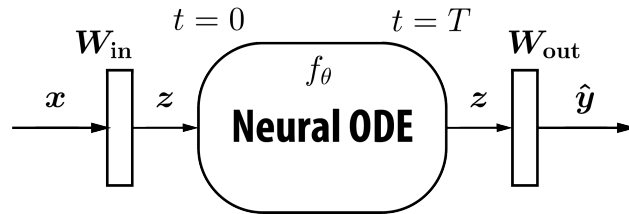

**Figure S2:** Schematic of the supervised learning architecture in Neural ODEs.

The feedforward phase begins at time  $t = 0$  with the input  $\mathbf{x}$  being mapped into the hidden state  $\mathbf{z}$  through the input projection layer  $W_{\text{in}}$ . Then,  $\mathbf{z}$  evolves from  $t = 0$  to  $t = T$  following the

dynamics specified by  $f_\theta$  (see Table S1 for the corresponding IVP). The final evolved hidden state  $\mathbf{z}(T)$  is then passed through the output projection layer  $W_{\text{out}}$  to obtain the network output  $\hat{\mathbf{y}}$ . This concludes the feedforward phase.

The feedback phase begins with computing the loss  $\mathcal{L}$  between  $\hat{\mathbf{y}}$  and  $\mathbf{y}$ . Instead of using the standard backpropagation algorithm like in FFNNs, which requires reverse propagating through the operations of the forward phase, the Neural ODEs framework computes loss gradients using the *adjoint sensitivity method*.<sup>6</sup> This method introduces a special *adjoint state* variable  $\mathbf{a}$ , defined as  $\mathbf{a} = \frac{\partial \mathcal{L}}{\partial \mathbf{z}}$ , which facilitates gradient computation by simultaneously solving three ‘backpropagation’ ODEs in reverse time (from  $t = T$  to  $t = 0$ ) to: (i) hidden state  $\mathbf{z}$  backpropagation, (ii) adjoint state  $\mathbf{a}$  backpropagation, and (iii) gradient  $\mathbf{g}_\theta$  evolution. The hidden state  $\mathbf{z}$  begins at its final feedforward state  $\mathbf{z}(T)$ , and flows backward to its initial state  $\mathbf{z}(0)$ , retracing its feedforward phase trajectory. The adjoint state  $\mathbf{a}$  starts from an initial value of  $\mathbf{a}(T) = \frac{\partial \mathcal{L}}{\partial \mathbf{z}}(T)$  and evolves into its final state at  $t = 0$ . The parameter gradients  $\mathbf{g}_\theta$  start from a zero initial value at  $t = T$  and evolve into their final values at  $t = 0$ . The simultaneous evolution of these three state variables ensures that the network evolves gradients alongside the variables it depends on, i.e.,  $\mathbf{a}$  and  $\mathbf{z}$ . The gradient values at the end of backpropagation ( $\mathbf{g}_\theta(0)$  at  $t = 0$ ) are used to update the parameters according to the gradient descent formulation (3).

The analog nature of the Neural ODEs framework makes it a more suitable reference for implementing chemical learning compared to the discrete FFNNs. For instance, increasing model complexity in FFNNs requires adding additional layers, which in turn introduces additional sequential steps, making the resulting one-pot reaction network implementation more cumbersome. In contrast, depth is defined in Neural ODEs by the  $T$  parameter, meaning that increasing model complexity doesn’t require more sequential steps, but rather involves running the same step for a longer duration. Moreover, the backpropagation algorithm in FFNNs necessitates storing the activations across hidden layers for adjoint backpropagation to compute gradients, leading to a significant memory overhead. In contrast, Neural ODEs avoid this overhead by simultaneously backpropagating the hidden state alongside its adjoint state, thus requiring only constant memory.

**Table S1:** Supervised learning procedure in the Neural ODEs framework consisting of seven steps. Each step can be classified into a ‘discrete’ (1, 3, 4, 5, 7) or ‘analog’ (2, 6) step based on the nature of its computations. ‘Analog’ steps are marked with an asterisk (\*). The discrete computations are shown as instantaneous, while analog computations take place over a time interval. Also, notice that the analog computations in step (6) take place in reverse-time.

| Step                                          | Description                   | Time               | ODE                                                                                           | IVP                                                                                                                          |
|-----------------------------------------------|-------------------------------|--------------------|-----------------------------------------------------------------------------------------------|------------------------------------------------------------------------------------------------------------------------------|
| 1                                             | Feeding the input             | $t = 0$            | $\mathbf{z}(0) = W_{\text{in}} \mathbf{x}$                                                    |                                                                                                                              |
| Feedforward Phase Begins                      |                               |                    |                                                                                               |                                                                                                                              |
| 2*                                            | Hidden state evolution        | $t = 0$ to $t = T$ | $\frac{d\mathbf{z}}{dt} = f_{\theta}(\mathbf{x}, \mathbf{z})$                                 | $\mathbf{z}(T) = \mathbf{z}(0) + \int_0^T f_{\theta}(\mathbf{x}, \mathbf{z}) \, dt$                                          |
| 3                                             | Output calculation            | $t = T$            | $\hat{y} = W_{\text{out}} \mathbf{z}(T)$                                                      |                                                                                                                              |
| Feedforward Phase Ends; Feedback Phase Begins |                               |                    |                                                                                               |                                                                                                                              |
| 4                                             | Loss calculation              | $t = T$            | $\mathcal{L} = \frac{1}{2}(\hat{y} - y)^2$                                                    |                                                                                                                              |
| 5                                             | Hidden state initialization   | $t = T$            | $\mathbf{z}(T)$ from the feedforward phase                                                    |                                                                                                                              |
|                                               | Adjoint initialization        | $t = T$            | $\mathbf{a}(T) \leftarrow \frac{\partial \mathcal{L}}{\partial \mathbf{z}}(T)$                |                                                                                                                              |
|                                               | Gradient initialization       | $t = T$            | $\mathbf{g}_{\theta}(T) \leftarrow \mathbf{0}$                                                |                                                                                                                              |
| 6*                                            | Hidden state backpropagation  | $t = T$ to $t = 0$ | $\frac{d\mathbf{z}}{dt} = f_{\theta}(\mathbf{x}, \mathbf{z})$                                 | $\mathbf{z}(0) = \mathbf{z}(T) + \int_T^0 f_{\theta} \, dt$                                                                  |
|                                               | Adjoint state backpropagation | $t = T$ to $t = 0$ | $\frac{d\mathbf{a}}{dt} = -\mathbf{a}^T \frac{\partial f_{\theta}}{\partial \mathbf{z}}$      | $\mathbf{a}(0) = \mathbf{a}(T) + \int_T^0 -\mathbf{a}^T \frac{\partial f_{\theta}}{\partial \mathbf{z}} \, dt$               |
|                                               | Gradient evolution            | $t = T$ to $t = 0$ | $\frac{d\mathbf{g}_{\theta}}{dt} = -\mathbf{a}^T \frac{\partial f_{\theta}}{\partial \theta}$ | $\mathbf{g}_{\theta}(0) = \mathbf{g}_{\theta}(T) + \int_T^0 -\mathbf{a}^T \frac{\partial f_{\theta}}{\partial \theta} \, dt$ |
| Feedback Phase Ends                           |                               |                    |                                                                                               |                                                                                                                              |
| 7                                             | Parameter update              | $t = 0$            | $\theta^{\text{new}} = \theta^{\text{old}} - \eta \mathbf{g}_{\theta}(0)$                     |                                                                                                                              |

### S3 Translating Polynomial ODEs into Deterministic CRNs

---

**Algorithm S1** Translation framework for converting a polynomial ODE into mass action CRNs

---

Let  $\mathcal{S} = \{x_1, x_2, \dots, x_n\}$  is a set of  $n$  real variables and  $f^P$  is a polynomial function defined on  $\mathcal{S}$ , then a polynomial ODE in  $\mathcal{S}$ :  $\frac{dx_i}{dt} = f^P(x_1, x_2, \dots, x_n)$  is translated into a deterministic CRN system as follows.

- 1: If the given ODE is a KDE, directly go to step 4.
  - 2: Each variable  $x \in \mathbb{R}$  is represented as a difference of two complementary positive-valued variables  $x^+, x^- \in \mathbb{R}^+$  ( $x = x^+ - x^-$ ) and the expressions in both left and right sides of the ODE are expanded. For simplicity, we assume that all the expressions are represented in the dual-rail notation.
  - 3: The ODE is segregated into two KDEs with positive monomials in the expansion assigned to a positive differential variable and negative monomials assigned to the negative differential variable.
  - 4: Each monomial is translated into a single chemical reaction in which the factor variable species become the reactants and the differential variable species becomes the product. Additionally, the reaction is assumed to be catalytic in all its reactants.<sup>7,8</sup> The coefficient of the monomial becomes the unitless rate constant of the reaction. This is referred to as the canonic mechanism.<sup>9</sup>
  - 5: Annihilation reactions are enabled between complementary dual-rail species, if present.
- 

### S4 Building Block CRNs in the Neural CRNs Framework

Below, we show the translation process for different classes of ODEs into CRNs, which will function as templates during the construction of the neural CRNs.

**Type-I-ODE.**  $\frac{dz}{dt} = xy$ , where  $x, y, z \in \mathbb{R}_{>0}$ , represents a Hungarian ODE with a single monomial term. The translation of this ODE into its corresponding chemical reaction is shown in Table S2.

**Table S2:** ODE to CRN translation of Type-I-ODE.

| ODE                                        | CRN                           |
|--------------------------------------------|-------------------------------|
| $\frac{dz}{dt} = xy, \quad x, y, z \geq 0$ | $X + Y \rightarrow Z + X + Y$ |

**Type-II-ODE.**  $\frac{dz}{dt} = xy$ , where  $x, y, z \in \mathbb{R}$ , is a non-Hungarian ODE system. Therefore it is first converted into a Hungarian system by rewriting it using dual-rail encoding. The resulting ODEs are

then independently translated into chemical reactions.

$$\begin{aligned}\frac{dz}{dt} &= xy \\ \frac{d(z^+ - z^-)}{dt} &= (x^+ - x^-)(y^+ - y^-) \\ \frac{dz^+}{dt} &= x^+y^+ + x^-y^- \\ \frac{dz^-}{dt} &= x^+y^- + x^-y^+\end{aligned}$$

where  $x^+, x^-, y^+, y^-, z^+, z^- > 0$ . Conversion to the dual-rail format results in four Type-I-ODEs, yielding four chemical reactions.

**Type-III-ODE.**  $\frac{dz}{dt} = -xy$ , where  $x, y, z \in \mathbb{R}$  follows a similar translation process as the Type-II-ODE as shown below:

$$\begin{aligned}\frac{d(z^+ - z^-)}{dt} &= -(x^+ - x^-)(y^+ - y^-) \\ \frac{dz^+}{dt} &= x^+y^- + x^-y^+ \\ \frac{dz^-}{dt} &= x^+y^+ + x^-y^-\end{aligned}$$

where  $x^+, x^-, y^+, y^-, z^+, z^- > 0$  results in four Type-I-ODEs and, by extension, yields four chemical reactions.

**Type-IV-ODE.**  $\frac{dz}{dt} = -z^2$ ,  $z \in \mathbb{R}$ , represents a Hungarian ODE that models the decay of  $z$ . Its CRN could be condensed into three reactions as shown below by allowing fast annihilation reactions between complementary dual-rail species.

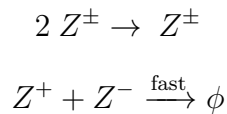

**Type-V-ODE.**  $\frac{dz}{dt} = z^2$ ,  $z \in \mathbb{R}^+$ , represents a Hungarian ODE that models the autocatalytic amplification of  $z$ . Its CRN could be similarly condensed into three reactions by allowing fast

annihilation reactions between complementary dual-rail species.

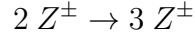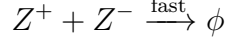

**CRNs for arithmetic operations.** Table S3 presents the CRNs (adapted from prior works<sup>10,11</sup>) for three algebraic operations used by the neural CRNs framework: (i) addition ( $y = a + b$ ),<sup>10</sup> (ii) subtraction ( $y = a - b$ ),<sup>10</sup> and (c) rational multiplication ( $y = wx$ ,  $w = \frac{p}{q}$ ,  $p, q \in \mathbb{Z}^+$  and  $\gcd(p, q) = 1$ ).<sup>11</sup> The addition CRN (`crn_add`) and subtraction CRN (`crn_subtract`) are both defined on real-valued variables, whereas the rational multiplication CRN (`crn_mult`) handles multiplication where one of the factors ( $w$ ) is rational.

**Table S3:** CRNs for arithmetic operations addition, subtraction, and rational multiplication.

| Addition ( <code>crn_add</code> ) | Subtraction ( <code>crn_subtract</code> ) | Multiplication ( <code>crn_mult</code> )           |
|-----------------------------------|-------------------------------------------|----------------------------------------------------|
| $A^+ \rightarrow Y^+$             | $A^+ \rightarrow Y^+$                     | $qX^+ \rightarrow pY^+$<br>$qX^- \rightarrow pY^-$ |
| $B^+ \rightarrow Y^+$             | $A^- \rightarrow Y^-$                     |                                                    |
| $A^- \rightarrow Y^-$             | $B^+ \rightarrow Y^-$                     |                                                    |
| $B^- \rightarrow Y^-$             | $B^- \rightarrow Y^+$                     |                                                    |

**CRN for the adjoint initialization.** The expected output  $\hat{y}$  is computed by applying  $W_{\text{out}}$  to the final hidden state  $z$  at the end of N1. Since the output is considered to be a scalar,  $W_{\text{out}}$  becomes a perceptron layer. Now, assuming that the weights are unit-valued  $w_i = 1$  and *squared loss* as the error function, we obtain the expression for adjoint as follows.

$$\hat{y} = w_1 z_1 + w_2 z_2 \tag{4}$$

$$\mathcal{L} = \frac{1}{2}(\hat{y} - y)^2 \tag{5}$$

$$\mathbf{a} = \frac{\partial \mathcal{L}}{\partial \mathbf{z}} \tag{6}$$

$$a_i = w_i(\hat{y} - y) \quad \text{using } w_i = 1 \tag{7}$$

$$\boxed{a_i = z_1 + z_2 - y} \tag{8}$$

Here,  $z_1$  and  $z_2$  have a positive feed into both the adjoint variables  $a_1$  and  $a_2$ , while  $y$  has the negative feed. Therefore, both the  $Z$  species of all parities should feed into the  $A$  species of their matching parity, while the  $Y$  species should feed into the  $A$  species of complementary parity. This CRN is represented as follows:

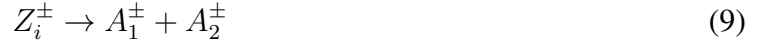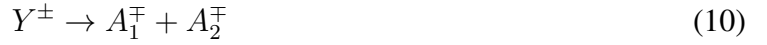

Finally, the subtraction is effected through annihilation reactions between complementary dual-rail species.

**CRN for gradient update.** The expression for gradient update:  $\theta^{\text{new}} = \theta^{\text{old}} - \eta g_\theta$  is a combination of multiplication and subtraction. These two operations can be represented using the following CRN

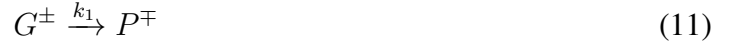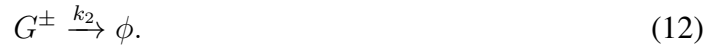

The opposite parity of  $G$  species feeding into the  $P$  species takes care of the subtraction, whereas the multiplication by  $\eta$  is covered by the relative ratio of  $k_1$  and  $k_2$ . Specifically,  $\eta = \frac{k_1}{k_1 + k_2}$ . Note that typical learning rates in machine learning are always  $\eta < 1$ . A simple assignment for  $k_1$  and  $k_2$  could be:

$$k_1 = \frac{\eta}{1 + \eta} \quad (13)$$

$$k_2 = \frac{1}{1 + \eta}. \quad (14)$$

Here, we provide a brief derivation for the above expressions.

Consider the two equations (15)

$$G \xrightarrow{k_1} P \quad (16)$$

$$G \xrightarrow{k_2} \Phi \quad (17)$$

$$\frac{dG}{dt} = -k_1 G - k_2 G \quad (18)$$

$$\frac{dP}{dt} = k_1 G \quad (19)$$

Substituting eq. (18), we obtain (20)

$$\frac{dP}{dt} = -\frac{k_1}{k_1 + k_2} \frac{dG}{dt} \quad (21)$$

Integrating on both sides from time  $t = 0 \rightarrow \infty$  (22)

$$\int_0^{P_f} \frac{dP}{dt} dt = -\frac{k_1}{k_1 + k_2} \int_{G_0}^0 \frac{dG}{dt} dt \quad (23)$$

$$\text{This gives: } P_f = \frac{k_1}{k_1 + k_2} G_0. \quad (24)$$

## S5 Linear regressor Neural CRN: Construction and Training

| Description                            | GitHub Link                                      |
|----------------------------------------|--------------------------------------------------|
| Branch for linear regression           | <a href="#">linear_regression</a>                |
| Permalink for dataset generation       | <a href="#">create_linear_regression_dataset</a> |
| Permalink for parameter initialization | <a href="#">create_node_params_reduced</a>       |
| CRN file                               | <a href="#">julia/linear_reduced2D.jl</a>        |

```
# CRN for the forward phase.
rn_dual_node_fwd = @reaction_network rn_dual_node_fwd begin
    # dz_i/dt = p_ix_i
    1.0, P1p + X1p --> Z1p + P1p + X1p
    1.0, P2p + X2p --> Z2p + P2p + X2p

    # dz_i/dt = h_i (h_i is constant and positive)
    1.0, H1p --> Z1p + H1p
    1.0, H2p --> Z2p + H2p
end

# CRN for the backpropagation phase.
rn_dual_node_bwd = @reaction_network rn_dual_node_bwd begin
    # Note: Doesn't require backpropagating z_i and a_i.
    # dg_i/dt = a_i x_i
    1.0, A1p + X1p --> G1p + A1p + X1p
    1.0, A1m + X1p --> G1m + A1m + X1p
    1.0, A2p + X2p --> G2p + A2p + X2p
    1.0, A2m + X2p --> G2m + A2m + X2p
end
```

**Listing 1:** Code for forward and backpropagation in the Linear Regressor Neural CRN

## S6 Nonlinear regression Neural CRN

### S6.1 Main nonlinear regression task ( $y = x_1x_2 + x_2^2$ )

| Description                            | GitHub Link                                     |
|----------------------------------------|-------------------------------------------------|
| Branch for nonlinear regression (main) | <a href="#">nonlinear_regression_z2_dotprod</a> |
| Main file to run                       | <a href="#">julia/neuralcrn_dotprod.jl</a>      |
| CRN file                               | <a href="#">julia/reactions_dotprod.jl</a>      |
| Execution                              | julia julia/neuralcrn_dotprod.jl                |

### S6.2 Task $y = x_1x_2 + x_2^2$ with first-order approximation of gradients

The simulation results are provided in Figure S3.

| Description                              | GitHub Link                                     |
|------------------------------------------|-------------------------------------------------|
| Branch (first order approx of gradients) | <a href="#">nonlinear_regression_z2_dotprod</a> |
| Main file to run                         | <a href="#">julia/neuralcrn_dotprod.jl</a>      |
| CRN file                                 | <a href="#">julia/reactions_dotprod.jl</a>      |
| Execution                                | julia julia/neuralcrn_dotprod.jl                |

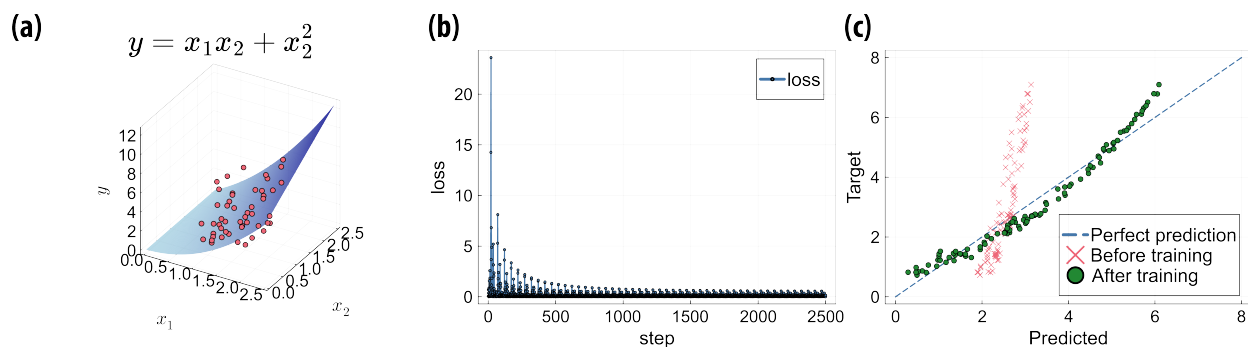

**Figure S3:** Results of simulating the nonlinear regression task  $y = x_1x_2 + x_2^2$  using a reduced nonlinear regression task.

```

# CRN for the forward phase.
rn_dual_node_relu_fwd = @reaction_network rn_dual_node_relu_fwd begin
    # dz_i/dt = h ('h' is constant and positive).
    1.0, H1p --> Z1p + H1p
    1.0, H1p --> Z2p + H1p
    1.0, H1p --> Z3p + H1p
    # dz_i/dt = p_ij x_j (x_j is considered to be positive)
    1.0, P11p + X1p --> Z1p + P11p + X1p
    1.0, P11m + X1p --> Z1m + P11m + X1p
    1.0, P22p + X2p --> Z2p + P22p + X2p
    1.0, P22m + X2p --> Z2m + P22m + X2p
    1.0, P33p + X3p --> Z3p + P33p + X3p
    1.0, P33m + X3p --> Z3m + P33m + X3p

    # Uses fast annihilation reactions.
    # dz_i/dt = -z_i^2
    1.0, 2Z1p --> Z1p
    1.0, 2Z1m --> Z1m
    100.0, Z1p + Z1m --> 0

    1.0, 2Z2p --> Z2p
    1.0, 2Z2m --> Z2m
    100.0, Z2p + Z2m --> 0

    1.0, 2Z3p --> Z3p
    1.0, 2Z3m --> Z3m
    100.0, Z3p + Z3m --> 0
end

# CRN for the backpropagation phase.
rn_dual_node_relu_bwd = @reaction_network rn_dual_node_relu_bwd begin
    # dg_ij/dt = a x
    1.0, A1p + X1p --> G11p + A1p + X1p
    1.0, A1m + X1p --> G11m + A1m + X1p
    1.0, A2p + X2p --> G22p + A2p + X2p
    1.0, A2m + X2p --> G22m + A2m + X2p
    1.0, A3p + X3p --> G33p + A3p + X3p
    1.0, A3m + X3p --> G33m + A3m + X3p
end

```

**Listing 2:** Code for forward and backpropagation in the Nonlinear Regressor Neural CRN

### S6.3 Task $y = \sin(x_1) + x_2^2$ with first-order approximation of gradients

The simulation results are provided in Figure S4.

| Description                              | GitHub Link                                            |
|------------------------------------------|--------------------------------------------------------|
| Branch (first order approx of gradients) | <a href="#">nonlinear_regression_z2_dotprod_sinxx2</a> |
| Main file to run                         | <a href="#">julia/neuralcrn_dotprod_simpler.jl</a>     |
| CRN file                                 | <a href="#">julia/reactions_dotprod_simpler.jl</a>     |
| Execution                                | julia julia/neuralcrn_dotprod_simpler.jl               |

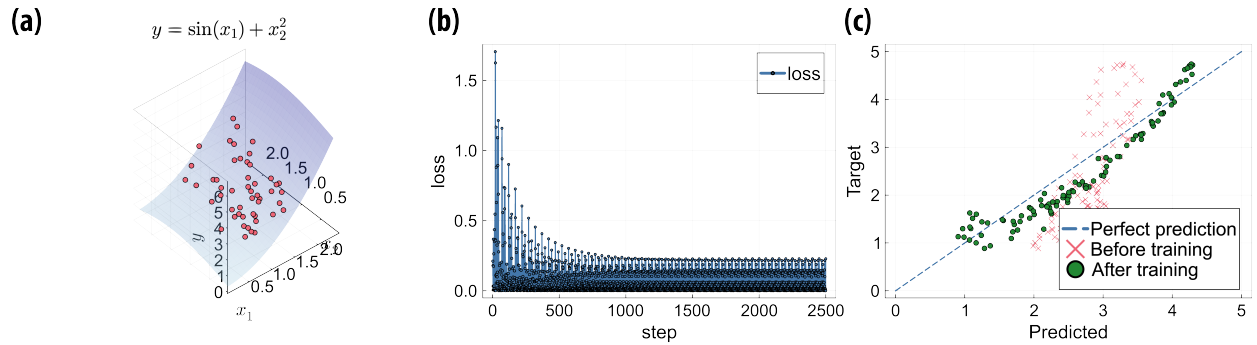

**Figure S4:** Results of simulating the nonlinear regression task  $y = \sin(x_1) + x_2^2$  using a reduced nonlinear regression task.

## S7 Proof of convergence stability for the hidden state dynamics

**function**  $f_{\theta,\beta}^{\text{cls}}$

For simplicity, we represent  $f_{\theta,\beta}^{\text{ncls}}$  as  $f$ . For the function  $f(\mathbf{x}, \mathbf{z}) = \theta\mathbf{x} + \beta - \mathbf{z} \odot \mathbf{z} \odot \mathbf{z}$  to be a valid hidden state dynamics function, the ODE

$$\frac{dz}{dt} = f(\mathbf{x}, \mathbf{z})$$

must be asymptotically stable. Without loss of generality, we consider the unidimensional case of the function and replace all terms independent of  $z$  with  $c$ . This simplifies the ODE to:

$$\frac{dz}{dt} = c - z^3 \quad (25)$$

The corresponding equilibrium points of the ODE are given by

$$\begin{aligned} c - z^{*3} &= 0 \\ z^* &= \sqrt[3]{c} \end{aligned} \quad (26)$$

### **S7.1 Proof of local asymptotic convergence stability**

To demonstrate local asymptotic stability, we show that the eigenvalues of the ODE's Jacobian have negative real parts. Given that the function is unidimensional, the Jacobian of the ODE and its eigenvalues both take the value of  $\frac{df}{dz}$ .

$$\frac{df}{dz} = -3z^2 < 0 \quad (27)$$

$$(28)$$

Since this value is always negative, we conclude that the ODE system is locally asymptotically stable.

### **S7.2 Proof of global asymptotic convergence stability**

We establish the global asymptotic stability of (25) by showing that the time derivative of the Lyapunov function is negative definite. We choose  $V(z)$  as the Lyapunov function.

$$V(z) = \frac{1}{2}(z - z^*)^2 \quad (29)$$

Computing its time derivative

$$\begin{aligned}\frac{dV(z)}{dt} &= \frac{dV(z)}{dz} \frac{dz}{dt} \\ \frac{dV(z)}{dt} &= (z - z^*)(c - z^3)\end{aligned}$$

Substituting  $z^* = \sqrt[3]{c}$  from (26), we obtain  $\frac{dV(z)}{dt} = (z - \sqrt[3]{c})(c - z^3)$

- $z > \sqrt[3]{c}, z^3 > c$  and  $\frac{dV(z)}{dt} < 0$
- $z < \sqrt[3]{c}, z^3 < c$  and  $\frac{dV(z)}{dt} < 0$

Thus,  $\frac{dV(z)}{dz} < 0 \forall z \neq \sqrt[3]{c}$ , demonstrating that the ODE system is globally asymptotically stable.

## S8 Nonlinear classification with neural CRNs

Here, we show the construction of the CRNs for the NLC-NCRN classifier using  $f_{\theta, \beta}^{nlcls} = \theta \mathbf{x} + \beta - \mathbf{z} \odot \mathbf{z} \odot \mathbf{z}$  as the activation function. The nature of this activation function is such that at steady state, it simulates the cube root of the linear transformation  $y = \theta \mathbf{x} + \beta$ .

$$\begin{aligned}f_{\theta, \beta}^{nlcls} &= \theta \mathbf{x} + \beta - \mathbf{z} \odot \mathbf{z} \odot \mathbf{z} \\ \frac{dz_i}{dt} &= (\theta \mathbf{x} + \beta)_i - z_i^3\end{aligned}$$

$$\text{Assume } y_i = (\theta \mathbf{x} + \beta)_i$$

$$z_i^{ss} = \sqrt[3]{y_i}$$

Here,  $\theta$  and  $\beta$  represent the parameters of the ODE system,  $\mathbf{x}$  represents the input,  $\mathbf{z}$  represents the ODE state variable, and  $\odot$  represents the element-wise (hadamard) product.

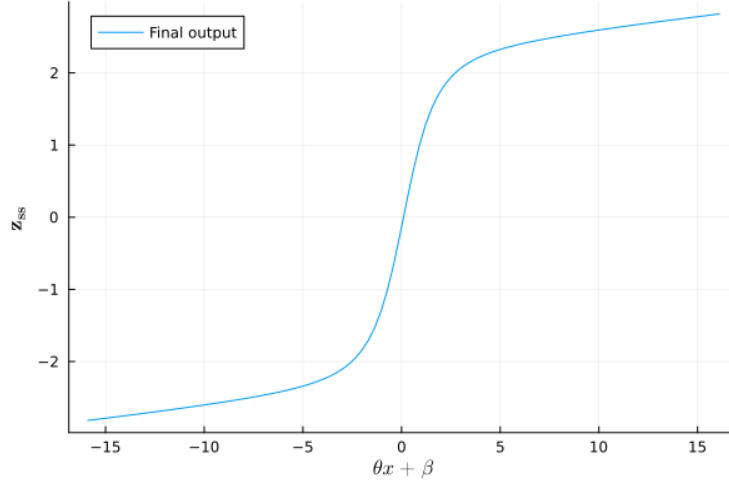

**Figure S5:** Activation function with the linear transformation  $\theta x + \beta$  on the X-axis and the associated activation computed by  $f_{\theta, \beta}^{nl}$  at the steady state on Y-axis.

Table S4 and Table S5 depict the forward and backward phase CRNs of the classifier, respectively.

**Table S4:** CRN for the forward stage of the Nonlinear Neural CRN.  $p_*$  represents the dual-rail parities of the species. The product  $\prod_i p_i$  represents the parity multiplication.

| Monomial                           | CRN                                                                                                        |
|------------------------------------|------------------------------------------------------------------------------------------------------------|
| $\frac{dz_i}{dt} = \theta_{ij}x_j$ | $P_{ij}^{p_\theta} + X_j^{p_x} \rightarrow Z_i^{p_\theta p_x} + P_{ij}^{p_\theta} + X_j^{p_x} + Z_i^{p_z}$ |
| $\frac{dz_i}{dt} = \beta_i$        | $B_i^{p_\beta} \rightarrow Z_i^{p_\beta p_z} + B_i^{p_\beta}$                                              |
| $\frac{dz_i}{dt} = -z_i^3$         | $3Z_i^\pm \rightarrow 2Z_i^\pm \quad (Z_i^+ + Z_i^- \xrightarrow{fast} \phi)$                              |

**Table S5:** Backpropagation CRNs for the NLC-NCRN.  $p_*$  represents the dual-rail parities of the species. The product  $\prod_i p_i$  represents the parity multiplication. The ‘bar’ on top of a parity represents the complement.

| Monomial                            | CRN                                                                                                                     |
|-------------------------------------|-------------------------------------------------------------------------------------------------------------------------|
| $\frac{dz_i}{dt} = -\beta$          | $B^\pm \rightarrow Z_i^\mp + B^\pm$                                                                                     |
| $\frac{dz_i}{dt} = -\theta_{ij}x_j$ | $P_{ij}^{p_\theta} + X_j^{p_x} \rightarrow Z_i^{\overline{p_\theta p_x}} + P_{ij}^{p_\theta} + X_j^{p_x}$               |
| $\frac{dz_i}{dt} = z_i^3$           | $3Z_i^\pm \rightarrow 4Z_i^\pm \quad (Z_i^+ + Z_i^- \xrightarrow{fast} \phi)$                                           |
| $\frac{da_i}{dt} = a_i z_i^2$       | $A_i^{p_a} + Z_i^{p_{z1}} + Z_i^{p_{z2}} \rightarrow A_i^{p_a p_{z1} p_{z2}} + A_i^{p_a} + Z_i^{p_{z1}} + Z_i^{p_{z2}}$ |
| $\frac{dg_{ij}}{dt} = a_i x_j$      | $A_i^{p_a} + X_j^{p_x} \rightarrow G_{ij}^{p_a p_x} + A_i^{p_a} + X_j^{p_x}$                                            |

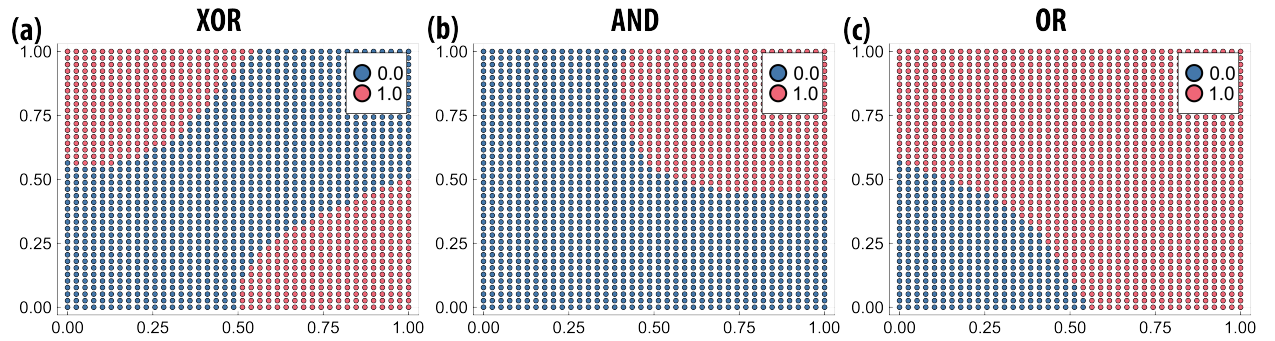

**Figure S6:** Visualized separation boundaries formed by the NLC-NCRN circuit on the XOR2D, AND2D, and OR2D datasets. The AND2D and OR2D datasets are designed similar to XOR2D described in the main text differing only in the Boolean function applied to assign the class label in the dataset.

## S9 Neural CRN for nonlinear classification with simplifications

This simplification is performed by removing the autocatalytic term in the backpropagation of

$$f_{\theta}^{\text{nclsV2}} = \theta \mathbf{x} - \alpha \mathbf{z} \odot \mathbf{z} \text{ corresponding}$$

| Description                            | GitHub Link                                                      |
|----------------------------------------|------------------------------------------------------------------|
| Branch (name is a misnomer)            | <a href="#">nonlinear_z3_linapprox</a>                           |
| Permalink for dataset generation       | <a href="#">create_xor_dataset</a>                               |
| Permalink for parameter initialization | <a href="#">create_node_params</a>                               |
| CRN file                               | <a href="#">julia/reactionsReLU.jl</a>                           |
| Command                                | <code>cd NeuralCRNGen &amp;&amp; julia julia/neuralcrn.jl</code> |

```
rn_dual_node_relu_fwd = @reaction_network rn_dual_node_relu_fwd begin
```

```
# dz_i/dt = p_i x_i
```

```
1.0, P11p + X1p --> Z1p + P11p + X1p
```

```
1.0, P11m + X1p --> Z1m + P11m + X1p
```

```
1.0, P12p + X2p --> Z1p + P12p + X2p
```

```
1.0, P12m + X2p --> Z1m + P12m + X2p
```

```
1.0, P13p + X3p --> Z1p + P13p + X3p
```

```
1.0, P13m + X3p --> Z1m + P13m + X3p
```

```
1.0, P21p + X1p --> Z2p + P21p + X1p
```

```
1.0, P21m + X1p --> Z2m + P21m + X1p
```

```
1.0, P22p + X2p --> Z2p + P22p + X2p
```

```
1.0, P22m + X2p --> Z2m + P22m + X2p
```

```
1.0, P23p + X3p --> Z2p + P23p + X3p
```

```
1.0, P23m + X3p --> Z2m + P23m + X3p
```

```
1.0, P31p + X1p --> Z3p + P31p + X1p
```

```
1.0, P31m + X1p --> Z3m + P31m + X1p
```

```
1.0, P32p + X2p --> Z3p + P32p + X2p
```

```
1.0, P32m + X2p --> Z3m + P32m + X2p
```

```
1.0, P33p + X3p --> Z3p + P33p + X3p
```

```
1.0, P33m + X3p --> Z3m + P33m + X3p
```

```
# dz_i/dt = - \alpha z^2
```

```
0.3, 2Z1p --> Z1p
```

```
0.3, 2Z1m --> Z1m
```

```
100.0, Z1p + Z1m --> 0
```

```
0.3, 2Z2p --> Z2p
```

```
0.3, 2Z2m --> Z2m
```

```
100.0, Z2p + Z2m --> 0
```

```
0.3, 2Z3p --> Z3p
```

```
0.3, 2Z3m --> Z3m
```

```
100.0, Z3p + Z3m --> 0
```

```
end
```

```
rn_dual_node_relu_bwd = @reaction_network rn_dual_node_relu_bwd begin
```

```
# dz/dt = -p_i x_i
```

```
1.0, P11m + X1p --> Z1p + P11m + X1p
```

```
1.0, P11p + X1p --> Z1m + P11p + X1p
```

```
1.0, P12m + X2p --> Z1p + P12m + X2p
```

```
1.0, P12p + X2p --> Z1m + P12p + X2p
```

```
1.0, P13m + X3p --> Z1p + P13m + X3p
```

```
1.0, P13p + X3p --> Z1m + P13p + X3p
```

```
1.0, P21m + X1p --> Z2p + P21m + X1p
```

```
1.0, P21p + X1p --> Z2m + P21p + X1p
```

```
1.0, P22m + X2p --> Z2p + P22m + X2p
```

```
1.0, P22p + X2p --> Z2m + P22p + X2p
```

```
1.0, P23m + X3p --> Z2p + P23m + X3p
```

```
1.0, P23p + X3p --> Z2m + P23p + X3p
```

```
1.0, P31m + X1p --> Z3p + P31m + X1p
```

```
1.0, P31p + X1p --> Z3m + P31p + X1p
```

```
1.0, P32m + X2p --> Z3p + P32m + X2p
```

```
1.0, P32p + X2p --> Z3m + P32p + X2p
```

```
1.0, P33m + X3p --> Z3p + P33m + X3p
```

```
1.0, P33p + X3p --> Z3m + P33p + X3p
```

```
# # dz_i/dt = \alpha z^2
```

```
#!!! Note that this part is removed as a simplifying approximation!!!
```

```
# 0.3, 2Z1p --> 3Z1p
```

```
# 0.3, 2Z1m --> 3Z1m
```

```
# 100.0, Z1p + Z1m --> 0
```

```

# 0.3, 2Z2p --> 3Z2p
# 0.3, 2Z2m --> 3Z2m
# 100.0, Z2p + Z2m --> 0

# 0.3, 2Z3p --> 3Z3p
# 0.3, 2Z3m --> 3Z3m
# 100.0, Z3p + Z3m --> 0

100.0, A1p + A1m --> 0
100.0, A2p + A2m --> 0
100.0, A3p + A3m --> 0

# # da_i/dt = -a_i z_i z_i
0.3, A1p + Z1m --> Z1m
0.3, A1p + Z1p --> Z1p

0.3, A1m + Z1p --> Z1p
0.3, A1m + Z1m --> Z1m

0.3, A2p + Z2m --> Z2m
0.3, A2p + Z2p --> Z2p

0.3, A2m + Z2p --> Z2p
0.3, A2m + Z2m --> Z2m

0.3, A3p + Z3m --> Z3m
0.3, A3p + Z3p --> Z3p

0.3, A3m + Z3p --> Z3p
0.3, A3m + Z3m --> Z3m

# dg_ij/dt = a x
1.0, A1p + X1p --> G11p + A1p + X1p
1.0, A1m + X1p --> G11m + A1m + X1p

1.0, A1p + X2p --> G12p + A1p + X2p
1.0, A1m + X2p --> G12m + A1m + X2p

1.0, A1p + X3p --> G13p + A1p + X3p
1.0, A1m + X3p --> G13m + A1m + X3p

```

```

1.0, A2p + X1p --> G21p + A2p + X1p
1.0, A2m + X1p --> G21m + A2m + X1p

1.0, A2p + X2p --> G22p + A2p + X2p
1.0, A2m + X2p --> G22m + A2m + X2p

1.0, A2p + X3p --> G23p + A2p + X3p
1.0, A2m + X3p --> G23m + A2m + X3p

1.0, A3p + X1p --> G31p + A3p + X1p
1.0, A3m + X1p --> G31m + A3m + X1p

1.0, A3p + X2p --> G32p + A3p + X2p
1.0, A3m + X2p --> G32m + A3m + X2p

1.0, A3p + X3p --> G33p + A3p + X3p
1.0, A3m + X3p --> G33m + A3m + X3p

```

end

**Listing 3:** CRN for feedforward and feedback phases using  $f_{\theta}^{\text{nlclsV2}}$

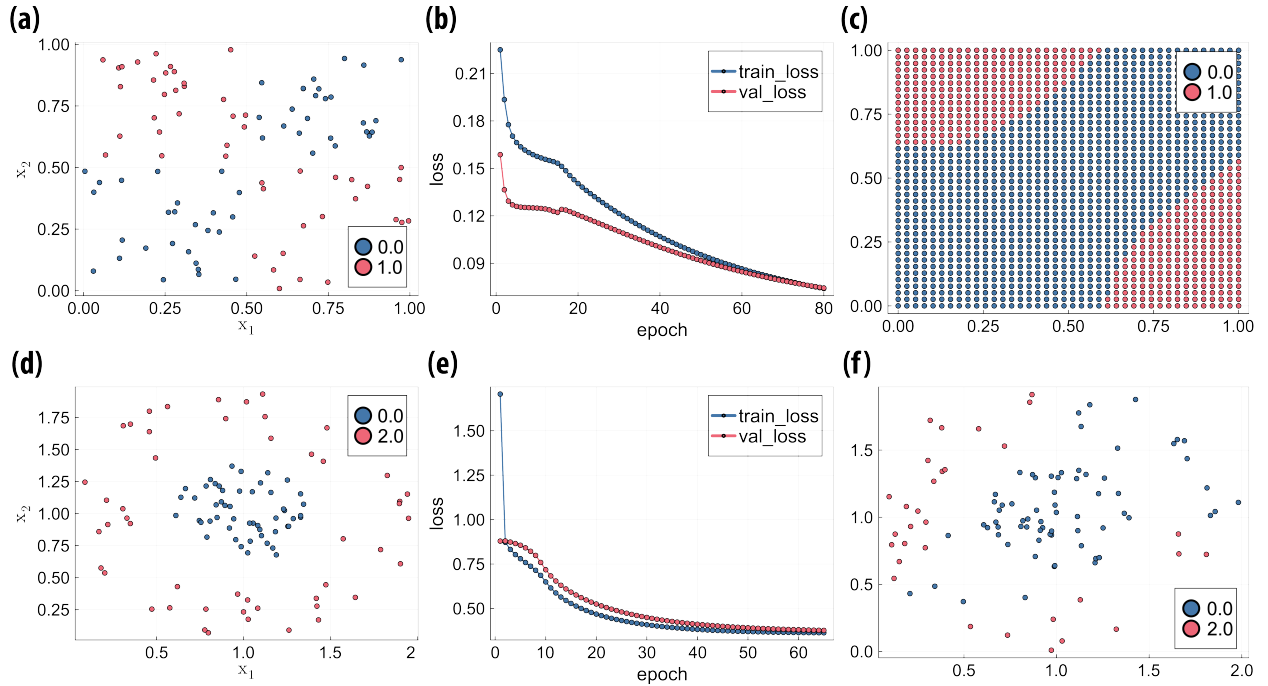

**Figure S7:** This simplification is performed by removing the autocatalytic term in the backpropagation of  $f_{\theta}^{\text{nlclsV2}} = \theta x + \beta - \alpha z \odot z$ , with  $\alpha = 0.3$ .

## S10 Multi-class classification

Here, we show how the binary classification architecture of neural CRNs described until now could be modified to support multi-class classification. In conventional machine learning architecture, it is possible to implement multi-class classification using binary classification models, one for each class, known as the ‘one vs all’ method, where a binary classifier is trained for the data points of each class against all the remaining classes. A straightforward method is to modify the final classification layer so that it takes in the final hidden state as input and outputs Here we will show how the prior binary classification architectures can be modified to support multi-class classification. First, we identify that the only difference between the two is the way the output is read out. The binary classification model employs the logistic regression formulation, where a single scalar output is interpreted as the class label by comparing it with a threshold. In contrast, the outputs of multi-class classification represent the individual class scores, with the highest-scoring class acting as the class label. The class labels are represented using *one-hot* encoding, i.e., as a binary vector with only one component in the ON state (as ‘1’) and the rest in the OFF state (as ‘0’). Consequently, the extension to multi-class classification could be easily performed by replacing the final layer in the prior architectures with a fully connected layer, with the size of output nodes equal to the class cardinality. No changes are required to core Neural CRN architecture, except for adjusting to the dimensionality of the classification task. We now validate our construction for multi-class classification using two real-world datasets: (i) the Iris dataset<sup>12</sup> and (ii) the Virus Infection dataset.<sup>13</sup>

**Iris.** The *Iris* dataset consists of the measurements of the width and length dimensions of the petal and sepal corresponding to the flowers of three different species in the *Iris* genus, namely *Iris-setosa*, *Iris-virginica*, and *Iris-versicolor*. It is a four-input dataset containing a total of 150 sample measurements divided equally among the three species, with each data point containing 4 real-valued features.

**Virus Infection.** The *Virus Infection* dataset is a small part of a larger collection NCBI GSE73032<sup>14</sup> with gene expression data of 12023 genes collected through micro-array assays from live human subjects. The subjects are inoculated separately with four respiratory viruses, viz., H1N1, H3N1, HRV, and RSV, and the gene expression values are measured at several time points before, during, and after inoculation. However, we only utilize a small subset of this dataset following the procedure suggested by.<sup>11</sup> Specifically, we collect gene expression data only at the disease *onset time*—the time point at which symptoms appear. Then, we utilize a random forest (RF) classifier (from Scikit-learn python package<sup>15</sup>) to select the top 9 genes from 12023, according to the feature importance scores provided by the RF classifier. The resultant dataset comprises 550 data points distributed unequally among the four classes.

For both the tasks (Iris and Virus Infection), the training set is constructed by randomly sampling 90% of the data points from each class, while the rest are put into the test set. Then, the training sets are subjected to min-max normalization, and the normalizing factors derived from the training set are used to normalize the test set. The nonlinear Neural CRN is trained in 5D augmented space for Iris (four features and one augmented dimension) and 10D augmented space for Virus Infection tasks (nine features and one augmented dimension). Figure S8 shows the Neural CRN architectures, validation accuracies at different stages of training, and inference schematic for the Iris and Virus Infection tasks, respectively. In both tasks, the trained model achieved an accuracy close to 1, indicating that our nonlinear Neural CRN model can perform multi-class classification with nonlinearly separable classes.

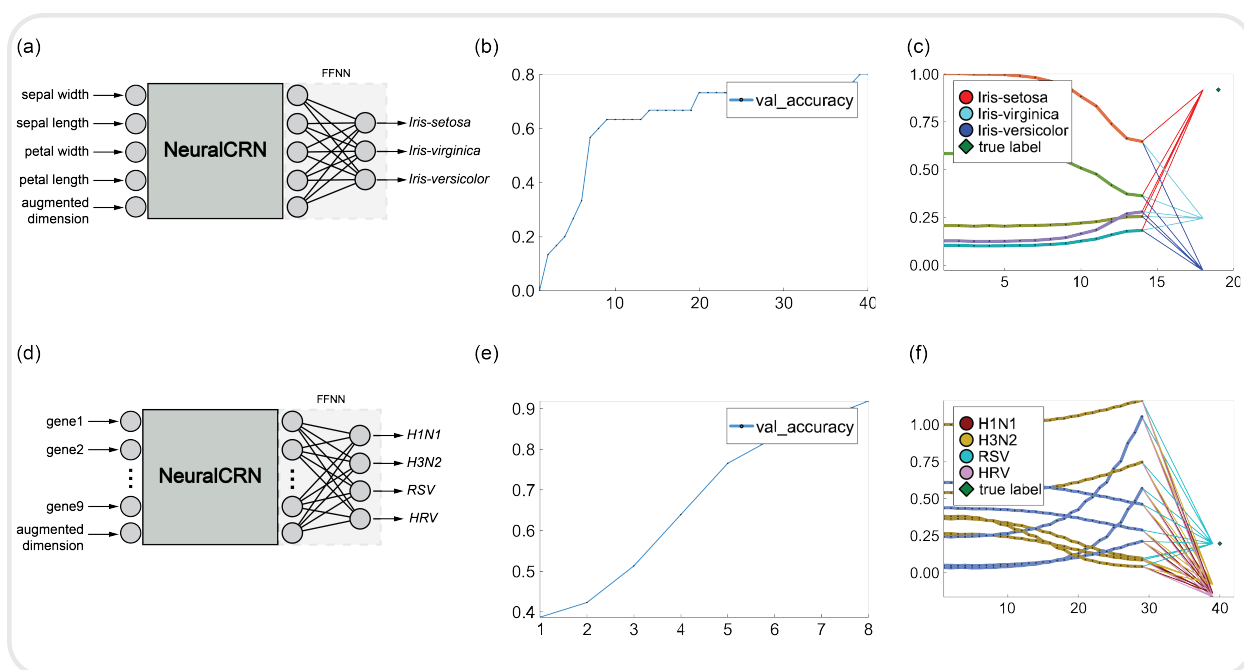

**Figure S8: Modeling multi-class classification in the neural CRNs framework.**

(a)-(c) correspond to the *Iris* dataset and (d)-(f) correspond to the *Virus Infection* dataset. (a, d) The Neural CRN architectures for training on the Iris and Virus Infection, respectively. It shows the input features and the class labels. The architecture differs from that of the binary classification architecture in that the outputs correspond to the class scores assigned by the model. The highest-scoring class is chosen as the prediction label. (b, e) Accuracy on the validation set as the training proceeds. The accuracy reaches close to 1, indicating that the training was successful. (c, f) Illustrations of the prediction process showing the Neural CRN "vector" flows (curved lines) and the weighted sum calculation at the classification layer (straight lines).

## S11 Parameter initialization for training the neural CRNs.

All the parameters are initialized using Xavier initialization.<sup>16</sup> The code below provides a general template for creating the requisite parameter and hyperparameters.

```
function create_params(dims; t0=0.0, t1=1.0, b=0.1)
    params = []

    # Dimensionality of the Neural CRN.
    push!(params, Float32(dims))

    # Theta parameters, Xavier initialization.
    theta = rand(Normal(0.0, 2.0), dims^2)
    theta = theta/sqrt(dims)
    append!(params, theta)

    # Beta parameters.
    beta = ones(dims)*b
    append!(params, beta)

    # Initializing all the weights to 1.
    w = ones(dims)

    # Begin and end times.
    push!(params, t0)
    push!(params, t1)

    return params
end
```

**Listing 4: Code for initializing the parameters through Xavier initialization.**

**Linear dataset.** For the *Linear* dataset, the theta parameters are chosen from the normal distribution  $\mathcal{U}(0, 2)$ , and the weight parameters are set to 1. The time range for the forward phase is set as follows:  $t_i = 0$  and  $t_f = 1.0$ . The learning rate is set to  $\eta = 1$ .

**Boolean datasets.** For all the *Boolean* datasets, the  $\theta$  parameters are chosen from the uniform distribution  $\mathcal{U}(0.0, 1.0)$ . The  $\beta$  parameters are all initialized to 0.1. The values of the augmented

dimensions  $AUGVAL$  are set to 0.2. The final layer weight parameters are constant and set to  $w_i = 1$ . The time range for the forward phase is set as:  $t_i = 0.0$  and  $t_f = 0.8$ . The learning rate is set to  $\eta = 1$ .

**Multi-class datasets.** For the *Iris* dataset, the  $\theta$  parameters are sampled from the normal distribution  $\mathcal{N}(0, 2)$  and Xavier normalization was performed. The  $\beta$  parameters are set to 0.1. The final layer weights are initialized, similar to the  $\theta$  initialization. Note that unlike the binary classification datasets above, the weights should be distinct in the multi-class setup as the outputs represent class scores. The value of  $AUGVAL$  is set to 1.0; the time range is set as follows:  $t_i = 0.0, t_f = 0.6$ ; and the learning rate is set to 0.01 [CODE]. The *Virus Infection* dataset follows the same initialization procedure except that the learning rate is set to  $\eta = 0.1$ .

## S12 Nonlinear Neural CRN with *ReLU* activation

For this, we utilize the nonlinear ODE system (30) developed by<sup>17</sup> that converges to a “smoothed” *ReLU* activated network at steady state as shown below:

$$\frac{dz}{dt} = h + (\theta \mathbf{x} + \beta) \odot \mathbf{z} - \mathbf{z} \odot \mathbf{z} \quad (30)$$

$$\text{Let } y = \theta \mathbf{x} + \beta \quad (31)$$

$$\lim_{t \rightarrow \infty} z_i = \frac{y + \sqrt{y^2 + 4h}}{2} \approx \text{ReLU}(y) \text{ as } h \rightarrow 0. \quad (32)$$

Here,  $h$  represents the smoothing constant,  $\theta$  and  $\beta$  represent the parameters of the ODE system,  $\mathbf{x}$  represents the input,  $\mathbf{z}$  represents the ODE state variable, and  $\odot$  represents the element-wise (hadamard) product. Note that  $y$  in (31) represents a hypothetical transformation via a linear neural network, and the steady-state value of  $z_i$  (32) is equivalent to applying a ‘smoothed’ *ReLU* activation to the output of a linear network, thus mimicking the operation of a *ReLU* network.

Table S6 represents the CRN for the forward phase. The  $p_*$  in the species’ superscript represents the species’ dual-rail parities, and the presence of multiple parities on a species represents parity multiplication.

**Table S6:** CRN for the forward stage of the Nonlinear Neural CRN.  $p_*$  represents the dual-rail parities of the species. The product  $\prod_i p_i$  represents the parity multiplication.

| Monomial              | CRN                                                                                                                        |
|-----------------------|----------------------------------------------------------------------------------------------------------------------------|
| $h$                   | $H^\pm \rightarrow Z_i^\pm$                                                                                                |
| $\theta_{ij} x_j z_j$ | $P_{ij}^{p_\theta} + X_j^{p_x} + Z_i^{p_z} \rightarrow Z_i^{p_\theta p_x p_z} + P_{ij}^{p_\theta} + X_j^{p_x} + Z_i^{p_z}$ |
| $\beta_i z_i$         | $B_i^{p_\beta} + Z_i^{p_z} \rightarrow Z_i^{p_\beta p_z} + B_i^{p_\beta} + Z_i^{p_z}$                                      |
| $-z_i^2$              | $2Z_i^\pm \rightarrow \phi \quad (\text{provided } Z_i^+ + Z_i^- \xrightarrow{\text{fast}} \phi)$                          |

Here, we show the equations ODEs and the CRNs for the backpropagation phase.

$$\frac{dz_i}{dt} = -\frac{dz_i}{dt} = -h - \theta_{i1}x_1z_i - \theta_{i2}x_2z_i - \theta_{i3}x_3z_i - \beta_iz_i + z_i^2 \quad (33)$$

$$\frac{d\mathbf{a}(t)}{dt} = -\mathbf{a}(t)^T \frac{\partial f}{\partial \mathbf{z}} = - \begin{bmatrix} a_1\theta_{11}x_1 + a_1\theta_{12}x_2 + a_1\theta_{13}x_3 - 2a_1z_1 \\ a_2\theta_{21}x_1 + a_2\theta_{22}x_2 + a_2\theta_{23}x_3 - 2a_2z_2 \\ a_3\theta_{31}x_1 + a_3\theta_{32}x_2 + a_3\theta_{33}x_3 - 2a_3z_3 \end{bmatrix} \quad (34)$$

$$\frac{d}{dt} \frac{\partial \mathcal{L}}{\partial \theta} = -\mathbf{a}(t)^T \frac{\partial f}{\partial \theta} = - \begin{bmatrix} a_1x_1z_1 & a_1x_2z_1 & a_1x_3z_1 \\ a_2x_1z_1 & a_2x_2z_2 & a_3x_2z_2 \\ a_3x_1z_1 & a_3x_2z_2 & a_3x_3z_3 \end{bmatrix} \quad (\text{Note: matrix reshaped for clarity}) \quad (35)$$

$$\frac{d}{dt} \frac{\partial \mathcal{L}}{\partial \beta} = -\mathbf{a}(t)^T \frac{\partial f}{\partial \beta} = - \begin{bmatrix} a_1z_1 & a_2z_2 & a_3z_3 \end{bmatrix} \quad (36)$$

Note that  $x_i$  here are the inputs and are thus constant. Observe that the monomials in the ODEs contain three factor variables instead of two, as in the prior case. This implies that the corresponding CRN reactions would be trimolecular, which increases the implementation complexity. The ODE to CRN translation follows a similar procedure illustrated in the template construction but with the presence of an extra variable. Note that the signs of the backpropagation ODEs (34) and (36) and (35) have to be inverted before converting them into CRNs. Table S7 presents the CRNs for the backpropagation phase.

**Table S7:** Backpropagation CRNs for the NLC-NCRN.  $p_*$  represents the dual-rail parities of the species. The product  $\prod_i p_i$  represents the parity multiplication. The ‘bar’ on top of a parity represents the complement.

| Monomial                               | CRN                                                                                                                                   |
|----------------------------------------|---------------------------------------------------------------------------------------------------------------------------------------|
| $\frac{dz_i}{dt} = -h$                 | $H^\pm \rightarrow Z_i^\mp$                                                                                                           |
| $\frac{dz_i}{dt} = -\theta_{ij}x_jz_i$ | $P_{ij}^{p_\theta} + X_j^{p_x} + Z_i^{p_z} \rightarrow Z_i^{\overline{p_\theta p_x p_z}} + P_{ij}^{p_\theta} + X_j^{p_x} + Z_i^{p_z}$ |
| $\frac{dz_i}{dt} = -\beta_i z_i$       | $B_i^{p_\beta} + Z_i^{p_z} \rightarrow Z_i^{\overline{p_\beta p_z}} + B_i^{p_\beta} + Z_i^{p_z}$                                      |
| $\frac{dz_i}{dt} = z_i^2$              | $2Z_i^\pm \rightarrow 3Z_i^\pm$                                                                                                       |
| $\frac{da_i}{dt} = a_i\theta_{ij}x_j$  | $A_i^{p_a} + P_{ij}^{p_\theta} + X_j^{p_x} \rightarrow A_i^{p_a p_\theta p_x} + A_i^{p_a} + P_{ij}^{p_\theta} + X_j^{p_x}$            |
| $\frac{dg_{ij}}{dt} = a_i z_i x_j$     | $A_i^{p_a} + Z_i^{p_z} + X_j^{p_x} \rightarrow A_i^{p_a p_z p_x} + A_i^{p_a} + Z_i^{p_z} + X_j^{p_x}$                                 |

## S13 Two-domain Strand Displacement Framework

While these frameworks can in theory simulate arbitrary CRNs, each is optimized for a specific set of chemical behaviors. As mentioned before, the CRNs in the neural CRNs architecture are noncompetitive and catalytic, with molecularity of the reactions increasing with the network complexity. For example, linear Neural CRN classifiers utilize bimolecular catalytic reactions, whereas the nonlinear NeuralCRN classifiers require trimolecular catalytic reactions. We contend that the two-domain framework (also referred to as the *Join-Fork* framework) is well-suited for implementing the neural CRNs. Figure S9 shows the implementation of a bimolecular catalytic reaction  $X + Y \rightarrow Z + X + Y$  in the Join-Fork framework. Each reaction in this framework translates into a two-stage pipeline: (i) the *Join* stage, where the reactant signals are consumed and (ii) the *Fork* stage, where the product signals are released. The Join-Fork framework is advantageous in this situation because the implementation complexity and the design overhead only increase linearly with the increase in both reactants and products of the CRN. For example, qualitatively, the conversion of a bimolecular reaction into a trimolecular reaction involves inserting an additional stem into the Join and Fork fuel gates and introducing the fuel signals corresponding to the additional reactants and products.

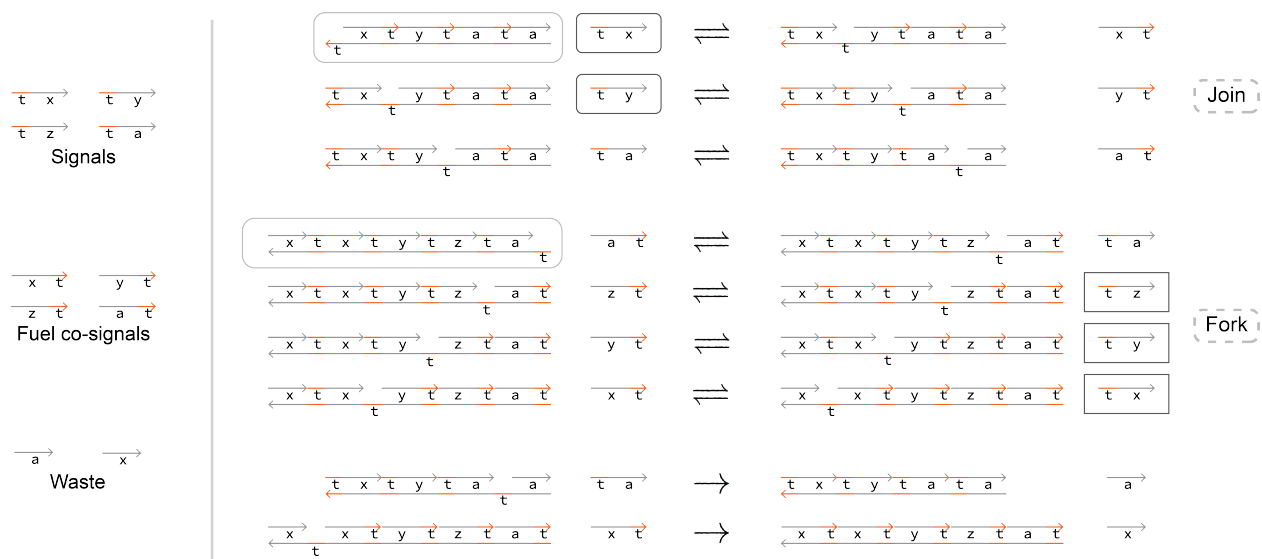

**Figure S9:** DNA strand displacement (DSD) reactions of the catalytic reaction  $X + Y \rightarrow Z + X + Y$  in the Join-Fork framework<sup>18</sup> This framework translates each abstract reaction into a two-stage pipeline: (a) *Join stage*—where the reactant signals (e.g.,  $X$  and  $Y$ ) are consumed, and (b) *Fork stage*—where the product signals (e.g.,  $Z$ ,  $X$ , and  $Y$ ) are released. Boxed species correspond to the raw materials for the reaction and the rest represent the intermediates. The side panel on the left depicts the fuel ‘co-signal’ strands which facilitate the release of their corresponding signal strands.

## S14 Implicit lifting in the Nonlinear Neural CRN

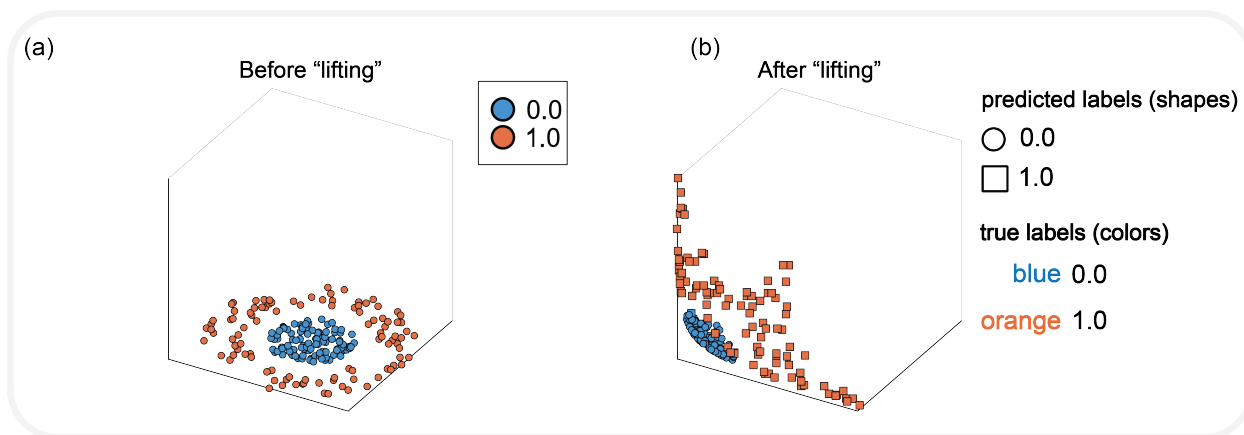

**Figure S10:** Implicit lifting visualized in the *Rings* dataset. (a) The data points that are not linearly separable in their original dimensionality (in this case, 2). (b) The data points become linearly separable by increasing the dimensionality (in this case, to 3) and applying a nonlinear transformation using the ‘smoothed’ *ReLU* dynamics function.<sup>17</sup>

## S15 Comparison of the parameter trajectories b/w LC-NCRN and an equivalent NeuralODE

In this section, we verify the construction of the linear Neural CRN by comparing its training behavior with that of a NeuralODE system. Specifically, we track the values of the four parameters  $\theta_{ij}, i, j \in \{1, 2\}$ . Note that since Neural CRN parameter values represent concentrations, they are all rounded off to two digits, whereas the NeuralODE parameters operate at the ‘Float32’ precision. Neural CRN parameter concentrations are all rounded off to 2 decimal digits so that they are a good representation of concentrations. Figure S11 presents the values of the algebraic variables (prefixed as “ode\_p”) and the concentrations of the Neural CRN parameter species (prefixed as “crn\_P”). In all the plots, we observe that the NeuralODE variables’ values and the corresponding Neural CRN concentrations correlate closely, validating our construction.

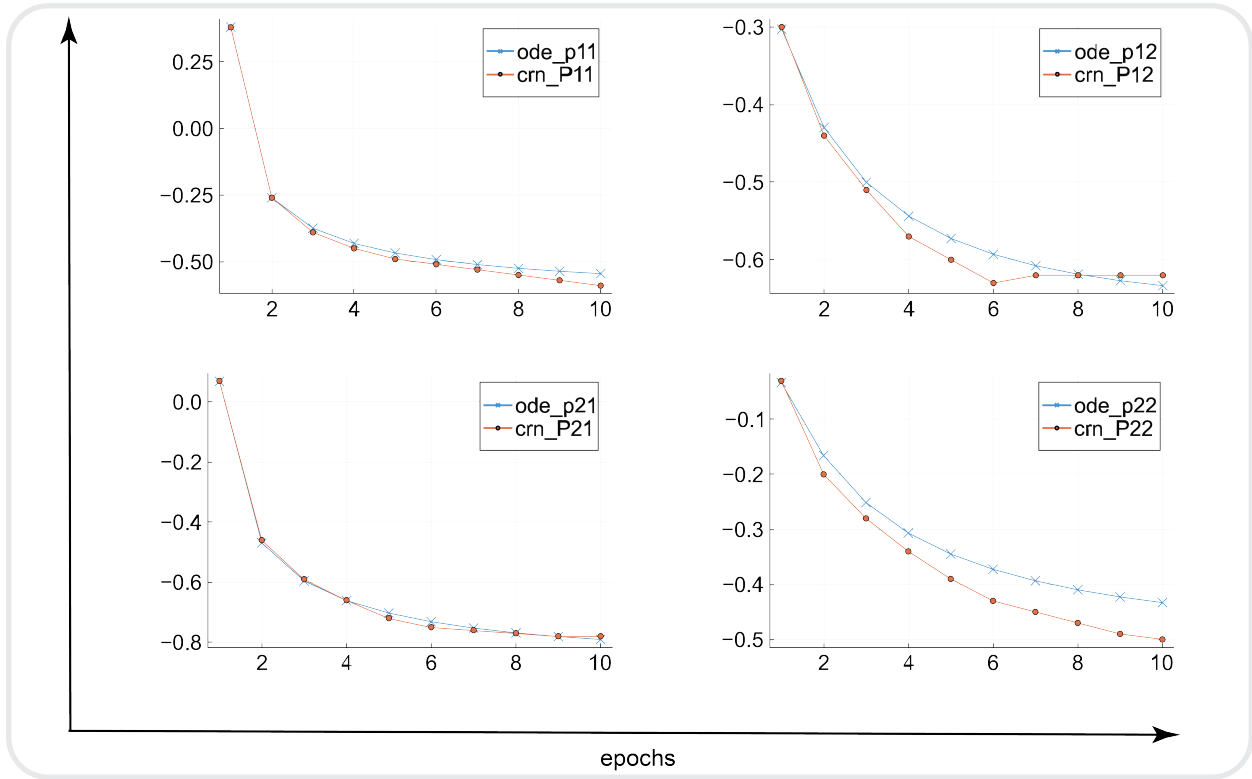

**Figure S11:** Compares the trajectories of the NeuralODE parameters (marked with a prefix “ode\_p”) and the concentration values of their corresponding Neural CRN parameters (marked with a prefix “crn\_P”).

## S16 Weight and Gradient trajectories for *Rings* dataset

Here, we present the weight and gradient trajectories for the *Rings* dataset with the model trained on the nonlinear Neural CRN described in the main text. Note that we only present a sample of the trajectories. We observe that the gradients converge to zero as the training proceeds, showing that the model learned to classify correctly. Note that the gradient trajectories are not of uniform scale on the Y-axis.

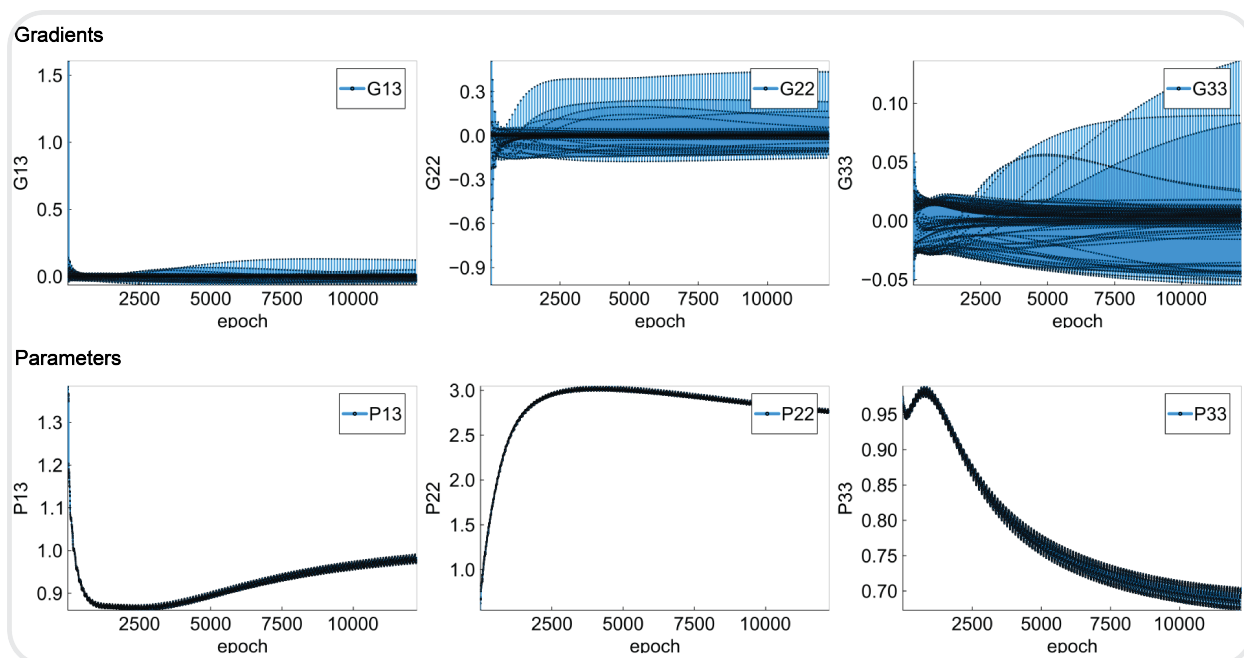

**Figure S12:** Gradient (top) and Parameter (bottom) trajectories of the *Rings* dataset during training. We observe that the gradients converge to zero as the training proceeds as expected.

## References

- (1) Rumelhart, D. E.; Durbin, R.; Golden, R.; Chauvin, Y. *Backpropagation: Theory, Architectures and Applications*; Lawrence Erlbaum Hillsdale, NJ, USA, 1995; pp 1–34.
- (2) Rumelhart, D. E.; Hinton, G. E.; Williams, R. J. Learning representations by back-propagating errors. *Nature* **1986**, *323*, 533–536.
- (3) Rall, L. B. *Automatic differentiation: Techniques and applications*; Springer, 1981.
- (4) Chen, R. T.; Rubanova, Y.; Bettencourt, J.; Duvenaud, D. K. Neural ordinary differential equations. *Advances in neural information processing systems* **2018**, *31*.
- (5) Hairer, E.; Wanner, G. Algebraically stable and implementable Runge-Kutta methods of high order. *SIAM Journal on Numerical Analysis* **1981**, *18*, 1098–1108.
- (6) Pontryagin, L. S. *Mathematical Theory of Optimal Processes*; CRC Press, 1987.
- (7) Cardelli, L.; Tribastone, M.; Tschaikowski, M. From electric circuits to chemical networks. *Nat. Comput.* **2020**, *19*, 237–248.
- (8) Oishi, K.; Klavins, E. Biomolecular implementation of linear I/O systems. *IET Systems Biology* **2011**, *5*, 252–260.
- (9) Hárs, V.; Tóth, J. On the inverse problem of reaction kinetics. *Qualitative theory of differential equations* **1981**, *30*, 363–379.
- (10) Buisman, H.; ten Eikelder, H. M.; Hilbers, P. A.; Liekens, A. M. Computing algebraic functions with biochemical reaction networks. *Artificial life* **2009**, *15*, 5–19.
- (11) Vasić, M.; Chalk, C.; Luchsinger, A.; Khurshid, S.; Soloveichik, D. Programming and training rate-independent chemical reaction networks. *Proc. Natl. Acad. Sci. U. S. A.* **2022**, *119*, e2111552119.

- (12) Fisher, R. A. Iris. UCI Machine Learning Repository, 1988; DOI: <https://doi.org/10.24432/C56C76>.
- (13) Liu, T.-Y.; Burke, T.; Park, L. P.; Woods, C. W.; Zaas, A. K.; Ginsburg, G. S.; Hero, A. O. An individualized predictor of health and disease using paired reference and target samples. *BMC Bioinformatics* **2016**, *17*, 47.
- (14) Host gene expression signatures of H1N1, H3N2, HRV, RSV virus infection in adults. 2016; <https://www.ncbi.nlm.nih.gov/geo/query/acc.cgi?acc=GSE73072>.
- (15) Pedregosa, F. et al. Scikit-learn: Machine Learning in Python. *Journal of Machine Learning Research* **2011**, *12*, 2825–2830.
- (16) Glorot, X.; Bengio, Y. Understanding the difficulty of training deep feedforward neural networks. *Proceedings of the thirteenth* **2010**,
- (17) Anderson, D. F.; Joshi, B.; Deshpande, A. On reaction network implementations of neural networks. *J. R. Soc. Interface* **2021**, *18*, 20210031.
- (18) Cardelli, L. Two-domain DNA strand displacement. *Math. Struct. Comput. Sci.* **2013**, *23*, 247–271.
